# Supplementary material for: PIVOT: Preference-based Intervention Vectors for Pedagogical Tutor Steering
Source: arXiv:2608.07509 source file (2026-06-29)
Supplement: Supplementary file 1 [file prompt_alpha_eval.tex]

\section{Prompt Alpha Eval}
\label{appen:prompt-alpha}
